# Supplementary material for: Properties of Minimizing Entropy
Source: arXiv:2112.03143 source file (2021-12-06)
Supplement: Supplementary file 1 [file appendix_old.tex]

\appendix


\section{Gradient of entropy $\ent$}

Consider a vector of non-negative reals, $z \in \mathcal{R}_{\geq 0}^{s}$, which represents the unnormalized probability mass of a discrete variable $X$ taking each of $s$ states. Then the normalized probabilities are given by $\prob(X = i) = \frac{z_i}{\sum_{j} z_{j}}$ and entropy $\ent$ by:
%
\begin{align}
    \ent(z) \triangleq - \sum_{i} \frac{z_i}{\sum_{j} z_{j}} \log  \frac{z_i}{\sum_{j} z_{j}}
\end{align}
%
Assume that our minimization procedure performs gradient descent by subtracting the first order derivative of $\ent(z)$ from each mass $z_{k}$. The gradient of entropy with respect to each mass is:
%
\begin{align}
\frac{\df \ent(z)}{\df z_{k}} &=   
\frac{\df}{\df z_{k}} \Bigg ( - \frac{z_k}{\sum_{j} z_{j}} \log  \frac{z_k}{\sum_{j} z_{j}}
- 
\sum_{i \neq k} \frac{z_i}{\sum_{j} z_{j}} \log  \frac{z_i}{\sum_{j} z_{j}} \Bigg ) \\
%
&= \frac{- \sum_{i \neq k } z_i }{ \big( \sum_{j} z_j \big)^2 } 
+ \frac{- \sum_{i \neq k } z_i }{ \big(\sum_{j} z_j \big)^2 } \log \frac{z_k}{ \sum_{j} z_j }
- 
\sum_{i \neq k} \bigg (  \frac{- z_i}{ \big( \sum_{j} z_j \big)^2} 
+ \frac{- z_i}{ \big( \sum_{j} z_j \big)^2} \log \frac{z_i}{ \sum_{j} z_j }\bigg ) \\
%
&= \frac{- \sum_{i \neq k } z_i }{ \big( \sum_{j} z_j \big)^2 } \Bigg ( 1 + \log \frac{z_k}{ \sum_{j} z_j } \Bigg ) 
- 
\sum_{i \neq k}  \frac{- z_i}{ \big( \sum_{j} z_j \big)^2} \bigg ( 1 + \log \frac{z_i}{ \sum_{j} z_j } \bigg )  \\
%
&= \frac{- \sum_{i \neq k } z_i }{ \big( \sum_{j} z_j \big)^2 } \Bigg (\log \frac{z_k}{ \sum_{j} z_j } \Bigg ) 
+ 
\sum_{i \neq k}  \frac{z_i}{ \big( \sum_{j} z_j \big)^2} \bigg ( \log \frac{z_i}{ \sum_{j} z_j } \bigg )  \\
%
&= 
\frac{1}{\big( \sum_{j} z_j \big)^2} \sum_{i \neq k} z_i \log \frac{z_i}{z_k}\\
%
&=  \frac{1}{\big( \sum_{j} z_j \big)^2} \sum_{i} z_i \log \frac{z_i}{z_k} \qquad  \bigg [ =\frac{1}{\big( \sum_{j} z_j \big)^2} \sum_{i} z_i \bigg( \log \frac{z_i}{\sum_{j} z_j} - \log \frac{z_k}{\sum_{j} z_j} \bigg ) \bigg ] \label{eq:h_grad}
\end{align}


\section{Gradient of expected number of unique states drawn $\uniq$}

Now consider a different quantity, the expected number of unique states, $\uniq$, obtained with $m$ draws of $X$. Let $I_i$ be 1 if we draw at least 1 sample from the $i^{th}$ state of $X$, and 0 if we draw none. Then: 
%
\begin{align}
    \uniq(z, m) &\triangleq  \ex\big[\sum_i I_i\big] = \sum_i \ex\big[I_i\big] \label{eq:lin} \qquad \text{(linearity of expectation)} \\
    &= \sum_i 0 P(I_i=0) + 1 P(I_i=1) \\
    &= \sum_i 1 - \bigg(1 - \frac{z_i}{\sum_{j} z_j}\bigg)^m
\end{align}
%
The gradient of expected number of unique states with respect to each mass is:
%
\begin{align}
  &\frac{d \uniq(z, m)}{d z_k} = \frac{d}{d z_k} \bigg ( 1 - \bigg(1 - \frac{z_k}{\sum_{j} z_j}\bigg)^m \bigg ) + \sum_{i \neq k} \frac{d}{d z_k} \bigg (  1 - \bigg(1 - \frac{z_i}{\sum_{j} z_j}\bigg)^m \bigg )\\
  %
  &= -m  \bigg(1 - \frac{z_k}{\sum_{j} z_j}\bigg)^{m-1} \frac{d}{d z_k} \bigg ( -\frac{z_k}{\sum_{j} z_j} \bigg ) + \sum_{i \neq k} -m  \bigg(1 - \frac{z_i}{\sum_{j} z_j}\bigg)^{m-1}  \frac{d}{d z_k} \bigg ( - \frac{z_i}{\sum_{j} z_j} \bigg ) \\
  %
    &= - m  \bigg(1 - \frac{z_k}{\sum_{j} z_j}\bigg)^{m-1} \frac{z_k - \sum_{i} z_i}{\big ( \sum_{j} z_j \big )^2}
    + \sum_{i \neq k} -m  \bigg(1 - \frac{z_i}{\sum_{j} z_j}\bigg)^{m-1} \frac{z_i}{\big ( \sum_{j} z_j \big )^2}
    \\
    %
    &= \frac{m}{\big ( \sum_{j} z_j \big )^2}  
    \sum_i z_i \bigg ( \bigg(1 - \frac{z_k}{\sum_{j} z_j}  \bigg)^{m-1}  -  \bigg(1 - \frac{z_i}{\sum_{j} z_j}  \bigg)^{m-1} \bigg ) \label{eq:u_grad}
\end{align}
%


\section{Effects of minimizing entropy $\ent$}

Consider taking one gradient step of minimizing entropy $\ent$ with respect to unnormalized masses $z$, $\tilde{z} = z - \eta \frac{d \ent}{d z}$.
The following results follow directly from the definition of $\frac{d \ent}{d z}$ in \cref{eq:h_grad}.

\begin{corollary} \label{thm:1}
\textbf{Condition for whether a state's mass decreases or increases.}
A necessary and sufficient condition for the gradient to be positive (i.e. the mass should be decreased to decrease entropy) is that the log mass should be less than the weighted average of all log masses:
%
\begin{align}
    \frac{\df \ent}{\df z_{k}} > 0 \leftrightarrow 
\log z_k
< 
\sum_{i} \frac{z_i}{\sum_j z_j} \log z_i \label{eq:dec_cond}
\end{align}
And vice versa for increase in mass.
\end{corollary}

\begin{corollary} \label{thm:2}
\textbf{Mass order is preserved and gaps are widened.} 
$\forall k, k': z_k < z_{k'}$, the decrease in mass $z_k$ will be larger than the decrease in $m_{k'}$:
\begin{align}
    \eta\frac{\df \ent}{\df z_{k}} > \eta\frac{\df \ent}{\df z_{k'}} 
    %
    \leftrightarrow 
    \sum_{i} z_i \log z_k < \sum_{i} z_i \log z_{k'}
    %
    \leftrightarrow \top
\end{align}
\end{corollary}

\begin{corollary} \label{thm:3}
\textbf{Unless the masses start as uniform, they are never uniform during entropy minimization.}
Follows directly from \cref{thm:2}.
\end{corollary}

\begin{corollary} \label{thm:4}
\textbf{Zero masses and probabilities stick to zero.}
\Cref{eq:dec_cond} is always true if $z_k = 0$, but $z$ is defined on the non-negative reals, so any state with probability 0 will always stay at probability 0. 
\end{corollary}


\begin{theorem} \label{thm:5}
\textbf{Condition for whether a state's probability decreases or increases, and quantity of change.}
Proved and need to type up.
\end{theorem}

\begin{corollary}
 \label{thm:6}
\textbf{Probability order is preserved and gaps are widened.}
This follows from \cref{thm:2}. Since mass order is preserved and widened, and the new probabilities are simply the new masses divided by a value that is constant across all indices.
\end{corollary}

\begin{corollary} \label{thm:7}
\textbf{State with the smallest non-zero mass and probability always decreases in both mass and probability, and vice versa for the largest mass.}
The result for decrease/increase in mass follows directly from \cref{thm:4}; the smallest non-zero mass (as well as any zero masses) will always have a positive gradient, and the largest mass will always have a negative gradient.
The result for probabilities follows from \cref{thm:5}.
\end{corollary}

\begin{corollary}\label{thm:8}
\textbf{Uniform distribution uniquely maximises entropy, non-unique one-hot distributions minimize it.}
These are the cases where $\forall k: \triangle  z_{k} = 0$: either when the masses are all equal so $\frac{d \ent}{d z} = \bar{0}$, or there is only one non-zero mass, in which case the non-zero mass has gradient 0 and the zeros have gradient $\infty$, staying clamped at 0. 
These are also when all the partial derivatives w.r.t. probabilities are 0. 
You can also prove these critical points using the Lagrangian.
\end{corollary}

\begin{theorem}\label{thm:9}
\textbf{The sum of masses $\sum_i z_i$ always decreases.} Proved and need to type up.
\end{theorem}

\begin{theorem}\label{thm:10}
\textbf{The decrease in the probability of the smallest mass is lower bounded by a value that is 1) $> 0$ and 2) increases with time, so we can compute this value at any iteration to obtain an upper bound on the number of timesteps left until the smallest mass becomes 0. This guarantees that minimizing entropy continuously successfully minimizes the number of non-zero probability states and does not get stuck.}
Proved and need to type up. This result can already be used to show minimizing entropy decreases a generalization bound that uses the number of non-zero probability states (however we do even better with the result on expected number of drawn states $\uniq$, which decreases a tighter bound).
\end{theorem}

\begin{corollary} \label{thm:gen_sum}
\textbf{Let vector $w$ be non-negative reals sorted in descending order, $w \in \mathcal{R}_{\ge 0}^s$, $\forall i: w_{i} > w_{i+1}$. Then the dot product of $w$ with any sorted descending vector of reals that sums to 0, $x \in \mathcal{R}^s, \forall i: x_{i} > x_{i+1}, \sum_i x_i = 0$, is positive.}

Let $A$ be the indices of all positive elements in $x$ and $B$ be the indices of all negative or zero elements in $x$.
\begin{align}
    \sum_i w_i \spa x_i &>0 \\
    \leftrightarrow \bigg ( \sum_{a \in A} w_a \spa x_a \bigg ) + \bigg ( \sum_{b \in B} w_b \spa x_b \bigg ) &> 0 \\
    \leftrightarrow 
     \overbrace{\bigg ( \sum_{a \in A} x_a\bigg ) }^{g_A > 0}  \overbrace{\bigg (  \frac{\sum_{a \in A} w_a \spa x_a}{\sum_{a \in A} x_a}\bigg ) }^{f_A > 0}  + 
    \overbrace{\bigg ( \sum_{b \in B} x_b \bigg )}^{g_B < 0}   \overbrace{ \bigg ( \frac{\sum_{b \in B} w_b \spa x_B}{\sum_{b \in B} x_b} \bigg ) }^{f_B > 0}  &> 0 \\
    \leftrightarrow 
    f_A \spa g_A &> - f_B \spa g_B \\
    \leftrightarrow 
    \frac{f_A}{f_B} &> - \frac{g_B}{g_A} \\
    \leftrightarrow 
    \frac{f_A}{f_B} &> \frac{g_A}{g_A} = 1 \leftrightarrow  \top
\end{align}
because $g_A + g_B = 0$ and $f_A > f_B$.
\hfill$\square$.

\end{corollary}

\begin{theorem}\label{thm:11_proof}
\textbf{Decreasing $\ent$ decreases $\uniq$.} 
Assume that $z$ is sorted from smallest to largest mass. This does not affect the value of $\ent$ or $\uniq$ which are order independent.
Let $p_i \triangleq \prob(X = i)$ be the probability of each state according to $z$. Let the probability of not picking each state be $q_i \triangleq 1 - p_i$. Define $\tilde{p}, \tilde{q}$ the same way for $\tilde{z} = z - \eta \frac{d \ent}{d z}$.

Case for $m=1$: $\uniq(z, 1) - \uniq(\tilde{z}, 1) = 0 \leftrightarrow \sum_i \tilde{q}_i - q_i = \sum_i (1 - \tilde{p}_i) - (1 - p_i) = 0 \leftrightarrow \top$.
Then for any $m > 1$, the expected number of unique draws $\uniq$ decreases when descending $\ent$ iff:
\begin{align}
    \uniq(z, m) - \uniq(\tilde{z}, m) &> 0 \label{eq:1} \\
    \leftrightarrow \sum_i 1 - q_i^m - (1 - \tilde{q}_i^m) &> 0 \\
    \leftrightarrow \sum_i \tilde{q}_i^m &> \sum_{i} q_i^m  \label{eq:2}  \\
    \leftarrow \sum_{i} \tilde{q}_i^m  > \sum_{i} q_i \spa \tilde{q}_i^{m-1} &\land \sum_{i} q_i \spa \tilde{q}_i^{m-1} > \sum_i q_i^m \label{e:two_terms}
\end{align}
%
Now we prove the truth of both conditions in \cref{e:two_terms}. For the first condition in \cref{e:two_terms}:
%
\begin{align}
    \sum_{i} \tilde{q}_i^m & > \sum_{i} q_i \spa \tilde{q}_i^{m-1} \\
    \leftrightarrow
    \sum_{i} \tilde{q}_i \spa \tilde{q}_i^{m-1} & > \sum_{i} q_i \spa \tilde{q}_i^{m-1} \\
    \leftrightarrow
    \sum_{i} \tilde{q}_i^{m-1} \spa (\tilde{q}_i  - q_i) &> 0 \label{e:part1}
\end{align}
%
Since $z$ is sorted in increasing order, so is $\tilde{z}$ (\cref{thm:2}), and therefore so are $p$ (\cref{thm:6}) and $\tilde{p}$. So $q, \tilde{q}$ are sorted in decreasing order. The change in probabilities, $\tilde{p} - p$, is sorted in increasing order from most negative to most positive (\cref{thm:6}), and sums to 0 because $\tilde{p}, p$ both sum to 0. $\tilde{q}  - q = - (\tilde{p} - p)$ so $\tilde{q}  - q$ is sorted in decreasing order and also sums to 0.
Since $\tilde{q}$ is soted in decreasing order, so is $\tilde{q}^{m-1}$. Therefore by \cref{thm:gen_sum}, \cref{e:part1} is true. 

For the second condition in \cref{e:two_terms}. Let $\mu \triangleq \frac{1}{s} \sum_i \tilde{q}_i^{m-1} - q_i^{m-1}$:
%
\begin{align}
    \sum_{i} q_i \spa \tilde{q}_i^{m-1} & > \sum_{i} q_i^m \\
    \leftrightarrow 
    \sum_{i} q_i \spa \tilde{q}_i^{m-1} & > \sum_{i} q_i \spa q_i^{m-1} \\
    \leftrightarrow 
    \sum_{i} q_i ( \tilde{q}_i^{m-1} - q_i^{m-1}) & > 0 \\
    \leftrightarrow 
    \bigg ( \sum_{i} q_i ( \tilde{q}_i^{m-1} - q_i^{m-1} - \mu)  \bigg) +  \mu\sum_{i} q_i & > 0
\end{align}
%
First term is positive by \cref{thm:gen_sum}. Second term is $\geq 0$ because $\sum_{i} q_i$ is positive and $\mu$ is positive or zero (proof by induction, i.e. assuming  \cref{eq:1} and therefore \cref{eq:2} for $m-1$).
\hfill$\square$.

\end{theorem}
